# Supplementary material for: Mid-Infrared Detectors and Imagers Integrating All-Group IV Nanowires
Source: arXiv:2310.07833 source file (2023-10-11)
Supplement: Supplementary file 1 [file customCommands_SI.tex]

% \renewcommand\thesection{S\arabic{section}}
\renewcommand\thesection{Supplementary Note \arabic{section}}
% \renewcommand\thesubsection{\thesection.\arabic{subsection}}
\renewcommand\thesubsection{S\arabic{section}.\arabic{subsection}}

% Bring the section title to the left
\titleformat{\section}{\raggedright\bfseries}{\thesection.}{.3em}{}
\titleformat{\subsection}{\raggedright\bfseries}{\thesubsection.}{.5em}{}
% \titleformat{\section}{\raggedright\bfseries}{S\arabic{section}.}{.3em}{}

% https://ctan.math.ca/tex-archive/macros/latex/contrib/titlesec/titlesec.pdf
\titlespacing\section{0pt}{*4}{*1.5}
\titlespacing\subsection{0pt}{*4}{*1.5}
\titlespacing\subsubsection{0pt}{*4}{*1.5}

\renewcommand{\bibname}{References}

\DeclareTOCStyleEntry[
  indent=1.5em,
  beforeskip=2pt,
  linefill=\hfill
]{tocline}{subsection}

% Modify figure name to put Figure S1 instead of Fig. 1
\renewcommand{\figurename}{Figure}
\renewcommand\thefigure{S\arabic{figure}}

% Modify table name to put Table S1 instead of Table 1
% \renewcommand{\tablename}{Table}
% \renewcommand\thetable{S\arabic{section}}
\renewcommand\thetable{S\arabic{table}}
\renewcommand{\theequation}{S\arabic{equation}}
\renewcommand{\eqref}[1]{Eq. \ref{#1}}
