# Supplementary material for: Mid-Infrared Detectors and Imagers Integrating All-Group IV Nanowires
Source: arXiv:2310.07833 source file (2023-10-11)
Supplement: Supplementary file 2 [file packages_SI.tex]

\usepackage{bm}
\usepackage{titlesec}
\usepackage{array}
% \usepackage[resetlabels,labeled]{multibib} % Required for multiple bibliographies. Remove if there is a single bibliography
% \newcites{SuppInfo}{SI References}
% % The empty suppNotes.bib file is necessary for multiple bibliographies to work, due to a bug in revtex

% \usepackage[table]{xcolor}
% \usepackage[floatfix]{float}
\usepackage{tocbasic}
% \usepackage[nottoc]{tocbibind}

\usepackage[resetlabels]{multibib}
\newcites{SI}{References}
